# Supplementary material for: Universality in human cortical folding across lobes of individual brains
Source: arXiv:1806.03504 ancillary file (2018-06-13)
Supplement: Supplementary file 1 [file SM.pdf]

# Supplementary Materials

## Suppl. Text A

In the following we report the regression results for the offset ($K_{Lobe}$) changes with age in the different lobes for healthy subjects.

In the HCP dataset we found, with a multiple linear regression (MLR) model of $K_{Lobe}$~age*lobe using the Matlab function fitlm(), that there is a significant main effect with lobe (p=0) and a significant interaction effect of age:lobe (p=2.0844e-05). This means the decrease in $K_{Lobe}$ with age is significantly different in both slope and offset between lobes.

In the IXI dataset, we made similar observations. The main effect with lobe was again significant (p=0), and so was the interaction effect age:lobe (p=1.1202e-15).

In the NKI dataset, we made similar observations. The main effect with lobe was again significant (p=0), and so was the interaction effect age:lobe (p=6.938e-05).

## Suppl. Text B

In the main manuscript Fig. 2 and 3, we showed mean values of slope and offset (grouped by age categories in the case of slopes). Here we show the raw data points to give the reader a full view of the data. We will also make the data available for download upon acceptance of the manuscript (see Suppl. Text F for details).

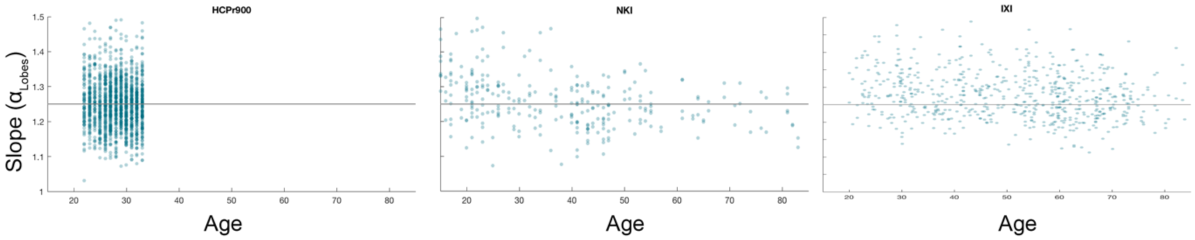


*Figure B.1:* Individual slopes ($\alpha_{Lobes}$) plotted against age in the HCP, NKI and IXI datasets. This is the underlying dataset for Fig. 2 in the main manuscript.

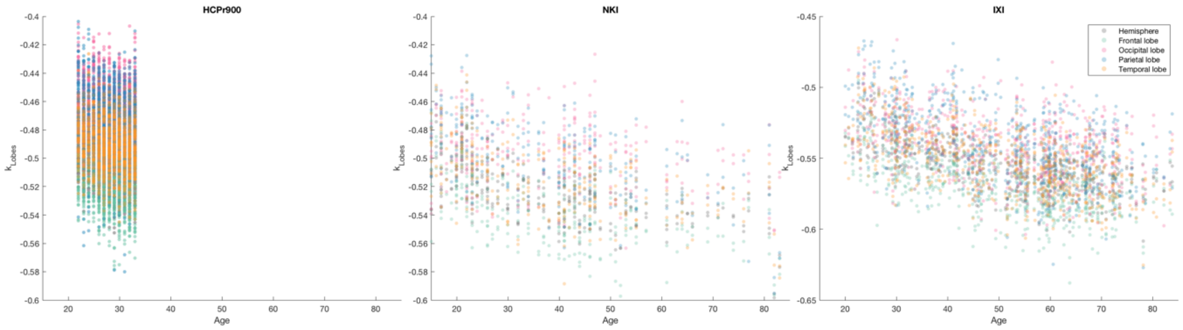


*Figure B.2:* Individual offset for each lobe of each hemisphere plotted against age in the HCP, NKI and IXI datasets. This is the underlying dataset for Fig. 3 in the main manuscript.

## Suppl. Text C

In the following we show how our slope obtained by regression across lobes of the same cortex, and fractal dimension of the cortex are related to the offset $K_{Hemisphere}$. If the scaling law is the only effect that drives cortical folding, then there is no reason for the slope or for the fractal dimension to show any relationship with the offset $K_{Hemisphere}$. However, in the following we will show that this relationship does exist, indicating that there may be secondary effects or scales that are currently assimilated in our offset parameter $K_{Hemisphere}$.

To estimate the fractal dimension, we used the code accompanying the paper [Madan2016] and available from https://github.com/cMadan/calcFD.

For each hemisphere, we calculated the fractal dimension, slope (based on lobes, $\alpha_{Lobes}$), and the $K_{Hemisphere}$ offset. We used the ADNI control participants between 60-70 years old, as a demonstration in the following two figures. The relationship between fractal dimension and $K_{Hemisphere}$ is particularly clear, but there is also a weak relationship between $\alpha_{Lobes}$ and $K_{Hemisphere}$.

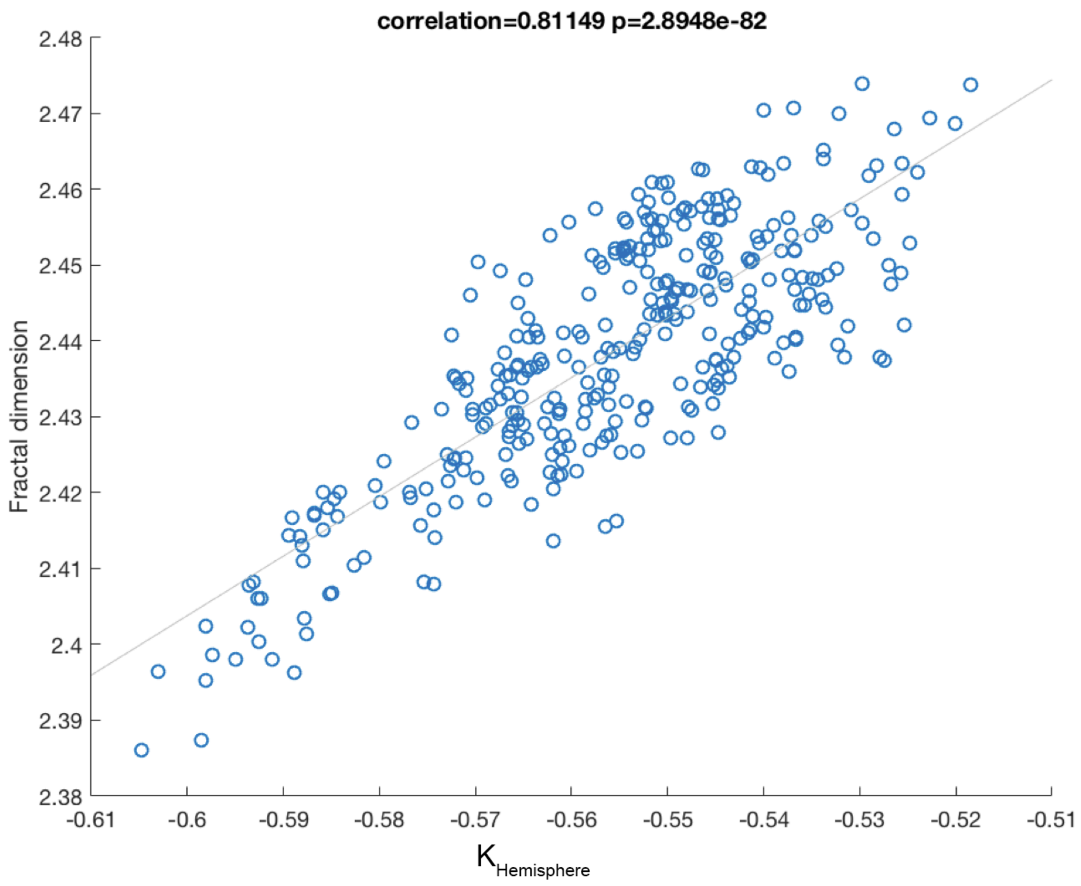

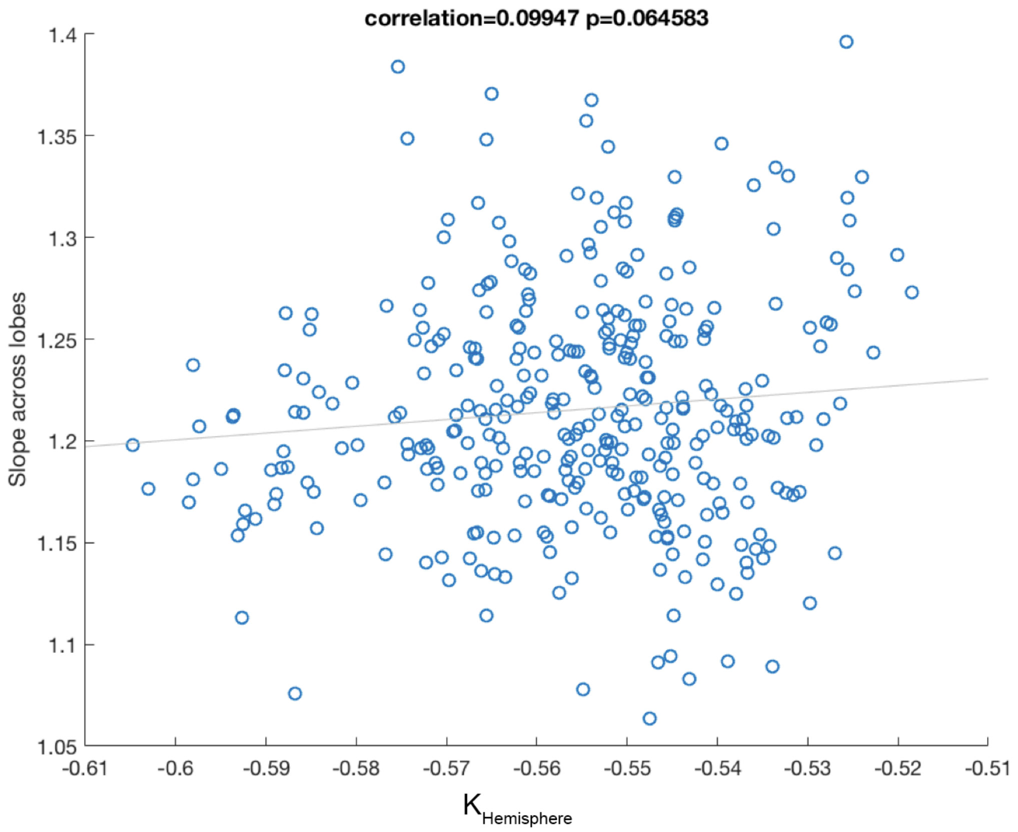


Note that the relationship between $K_{Hemisphere}$ and $\alpha_{Lobes}$ becomes more apparent when including a broader age range. The following figures shows the same relationship for the NKI data:

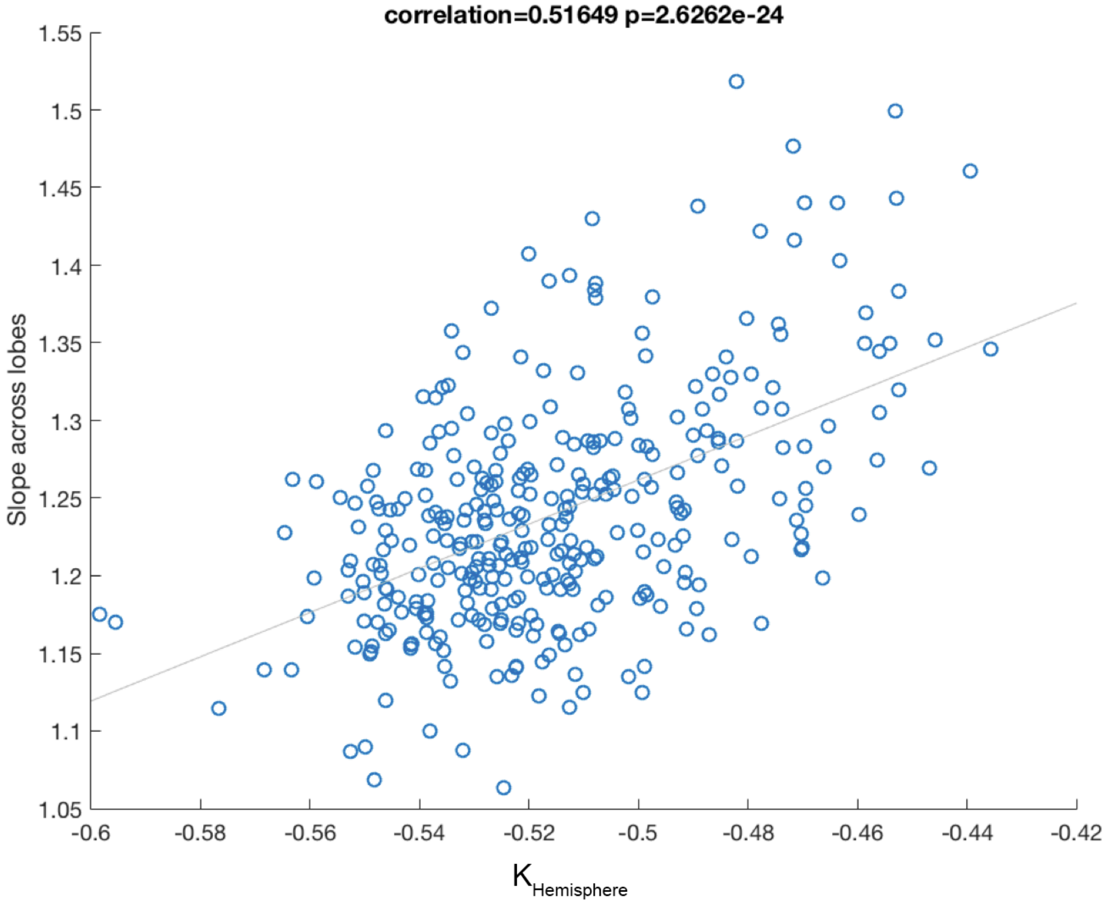


Qualitatively similar results are found for other datasets and age ranges. Hence, we believe that the trend in Fig. 2 in the main text of the slope changing slightly with age is actually not indicating that the mechanism of folding changes over age. Rather we think that there may be a secondary scale/effect with age that modulates our scaling law slightly.

Future work will have to elucidate what the secondary effects/scales are, and how these affect particularly the fractal dimension and also our slope estimates $\alpha_{Lobes}$.

[Madan2016] Madan, C. R., & Kensinger, E. A. (2016). Cortical complexity as a measure of age-related brain atrophy. NeuroImage, 134, 617-629. doi:10.1016/j.neuroimage.2016.04.029

## Suppl. Text D

In the following we compare AD and healthy controls in terms of how $K_{Lobe}$ (offset) and cortical thickness change over age for different lobes. Generally similar trends can be seen in both offset and thickness.

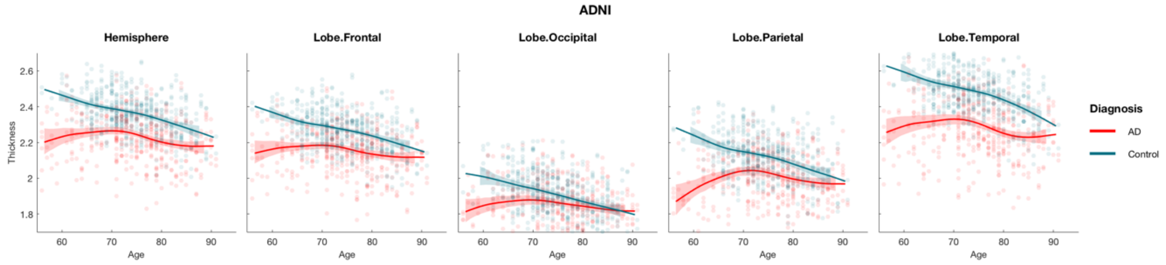


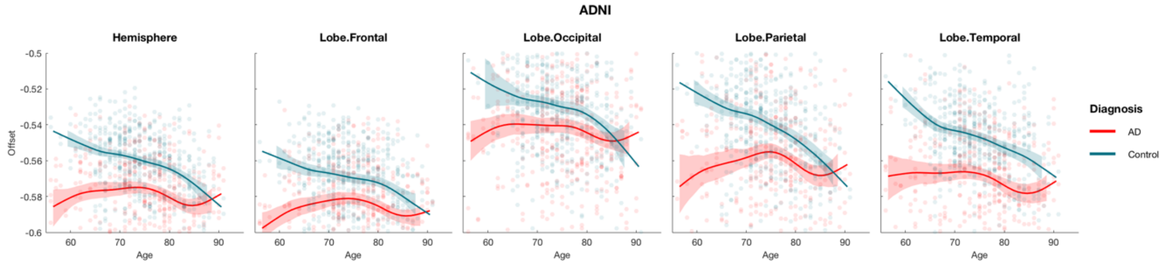


Solid lines indicate mean, and shaded areas indicate 95% bootstrapped confidence intervals of the mean.

The corresponding effects sizes between the AD and healthy controls are:

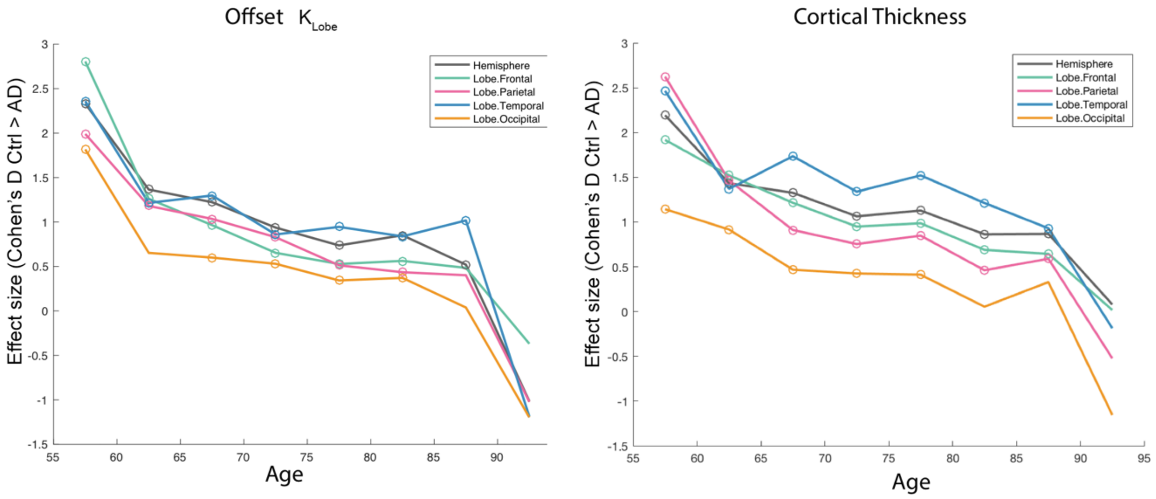

## Suppl. Text E

In this part, we provide the full details of how we partitioned cortical hemispheres into lobes, why a correction term for the Ae and At of the lobes is needed, how we estimated it, and how we then derived a slope for a hemisphere.

### Partition into lobes

To partition the cortex into lobes, we used the Freesurfer Desikan-Killiany parcellations and followed the Freesurfer suggestions for assigning them to the four lobes:

Frontal

- Superior Frontal
- Rostral and Caudal Middle Frontal
- Pars Opercularis, Pars Triangularis, and Pars Orbitalis
- Lateral and Medial Orbitofrontal
- Precentral
- Paracentral
- Frontal Pole
- Rostral Anterior Cingulate
- Caudal Anterior Cingulate

Parietal

- Superior Parietal
- Inferior Parietal
- Supramarginal
- Postcentral
- Precuneus
- Posterior Cingulate
- Isthmus

Temporal

- Superior, Middle, and Inferior Temporal
- Banks of the Superior Temporal Sulcus
- Fusiform
- Transverse Temporal
- Entorhinal
- Temporal Pole
- Parahippocampal

Occipital

- Lateral Occipital
- Lingual
- Cuneus
- Pericalcarine

We also included the insular cortex in our analysis for completeness. We assigned a portion of the insula to each the frontal, temporal and parietal lobe depending on the relative surface area of those lobes. In other words, if the frontal lobe surface area makes up 50%, the

temporal lobe makes up 30% and the parietal lobe makes up 20% of the summed surface area of the three lobes, then those percentages of the insular cortex are added to each lobe.

Note that the results do not change significantly if we do not include the insula, or if we assign it to different lobes according to some predefined percentages. The addition of the insular cortex is important only for completeness, and to ensure that the surface areas of all lobes add up to the total surface area of the cortex.

### Correction term for $A_e$ and $A_t$ of the lobes

In the main text, we explained that simply using the raw measures ($A_e$, $A_t$) of the partitions of the cortex is not necessarily going to provide any insight into how the partitions scale. Visualised in a log $A_e/T^2$ vs. log $A_T/T^2$ plot (see schematic in Fig. E.1, part A), a single cortical hemisphere, represented by the large black dot, would lie along the red line of slope 1.25 (of its group, which we did not visualise). However, if one divides this cortical hemisphere into two identical halves, each half would have the same average thickness and gyrification as the whole, but only half the total and exposed area. In the plot, they would coincide at the blue square along the blue line with slope one (each such parallel corresponds to a different value for the gyrification index $g=A_t/A_e$), intersecting the red line at the point corresponding to the whole cortex. The two halves (empty blue square) are shifted to the left and down from whole cortex by factors of log2 (as we halved the hemisphere). Further dividing a half cortex into identical quarters would only place each quarter further down along the blue line. Thus, a set of cortical hemispheres of different sizes would upon partitioning be distributed along the slope 1 direction even for homogeneous cortices.

Of course, the preceding thought experiment presumes a largely homogeneous cortical hemisphere, such that all partitions of equal size, large enough to include several gyri and sulci, would be substantially identical. But our objective here is precisely to determine if some version of the universal scaling law is preserved for different parts of the hemisphere even if they are substantially different from one another. For a partition of an inhomogeneous cortical hemisphere (see Fig. E.1, part B), each partition will naturally disaggregate according to its gyrification index (i.e., which blue lines) and size (i.e., how far down along the blue line). As previously, in the figure the black dot on the red line indicates the full cortical hemisphere. The two empty squares mark two dissimilar partitions of the full cortex, lying along the light blue lines corresponding to the gyrification index of each. For each partition, the distance along the line of constant gyrification index to the red line is determined by its size, relative to the whole hemisphere. Note that the size and gyrification index fully determine the position of these data points. Two similarly sized partitions with different gyrification indices could thus have a near infinite slope between them. Hence, we cannot expect a single scaling law to emerge when simply using the raw values of $A_e$ and $A_t$; there is no natural way to compare the area values from different partitions to each other and to the whole hemisphere.

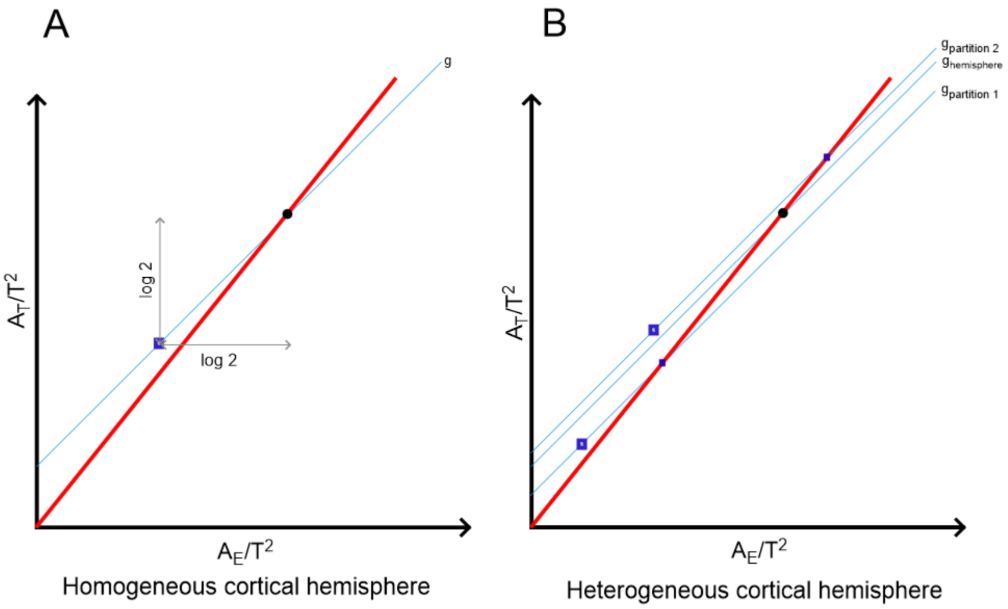


*Figure E.1 Morphological parameters for the whole cortex (dark dot) and its two partitions (empty squares). The red line correspond to the universal scaling relation. Blue lines correspond to constant values of the gyrification index $g=A_t/A_e$.*

What is needed then, is a self-consistent procedure for virtually reconstructing for each partition an equivalent datapoint for a full cortical hemisphere, while retaining its morphological characteristics: the average thickness T and the gyrification index g. The value of the total and exposed areas of this virtual cortex, $A_t'$ and $A_e'$, would then be the corrected area values for the partition, with the partition size effect removed and directly comparable to each other and to the whole hemisphere.

Of course, since we are only interested in $A_t'$ and $A_e'$, there is no need to produce an actual detailed reconstruction. Rather, for both the exposed and the total surfaces we require simply a ratio that quantifies the proportion of the reconstructed hemisphere that the partition corresponds to. A natural candidate for such a quantity is the ratio between the integrated Gaussian curvatures in the surface in question for the whole hemisphere (a topological invariant - 4π - for a closed surface) and the partition (where it is insensitive to small deformations). The values of $A_t'$ and $A_e'$ are then simply the original values for the areas in the partition times this ratio. As a consequence of this, the average Gaussian curvature is preserved. We can thus sum up our procedure by stating that the corrected total and exposed areas for a partition of a complete cortical hemisphere are the total and exposed areas of a complete hemisphere that has the same average thickness, gyrification index and average gaussian curvature as the corresponding surface in the partition.

$$\mathrm{T}'^{\mathrm{P}} = \mathrm{T}^{\mathrm{P}}$$

$$\mathrm{g}'^{\mathrm{P}} = \frac{A_t'^P}{\mathrm{A}_\mathrm{e}'^\mathrm{P}} = \frac{A_t^P}{A_e^P} = g^P$$

$$\bar{G}'^P_e = \frac{4\pi}{\mathrm{A}_\mathrm{e}'^\mathrm{P}} = \frac{I_G^P}{A_e^P} = \bar{G}_e^P$$

$$\bar{G}'^P_t = \frac{4\pi}{A_t'^P} = \frac{I_G^P}{A_t^P} = \bar{G}_t^P$$

(This is eq. 2 from the main text.)

After applying our correction, we essentially map those datapoints marked by empty squares to the datapoints marked by filled squares in Fig. E.1B. Since the correction preserves both T and g, the mapping occurs along the lines of constant gyrification index. In this schematic (Fig. E.1) the corrected values of log $A_e$ and log $A_t$ can be fitted linearly, and the resulting slope compared to the expected 1.25. Note that at no point we enforced this expected value, rather it emerges independently as a consequence of our correction term.

Note finally that by "reconstructed cortex", we do not mean producing a detailed surface description of a new cortical hemisphere, but simply a computation of the morphological variables $A^P_e$ and $A^P_t$ that such reconstructed cortex would have to allow for comparisons in the terms of Equation (1). We denoted the reconstructed variables with ' throughout the main manuscript.

## Estimation of $I_G^P$

To estimate the curvature density, we used the triangulation of the exposed surface of the partition (obtained from the Freesurfer, see Suppl Text F). Ideally, this surface would be convex. In reality, it may have small concavities, which have negative curvature. The value of the total Gaussian curvature for a partition can be extremely sensitive to the precise placing of its boundary if it crosses an area of concentrated negative curvature. To rectify this, we calculated the convex hull of the exposed surface of the partition. We then obtained the integrated Gaussian curvature of the convex hull and used this as $I_G^P$. Being a topological invariant (i.e., insensitive to continuous transformations of shape), the integrated gaussian curvature of the smooth closed cortical surface is exactly the same as that of its convex hull and of its triangulated representation. To a very good approximation the same is true for partitions of the whole cortical surface, as long as the partitions are large enough. For triangulated surfaces, all the curvature is concentrated on the vertices, with a value in each being the difference between $2\pi$ and the sum of incident angles of the attached faces. Using the convex hull to calculate $I_G^P$ has the further advantage of only evaluating the Gaussian curvature at a small number of triangulation points, and thus reduces the numerical estimation errors. This so-called topological invariant is thus a natural measure of the relative sizes of different partitions of a closed surface that is insensitive to deformations and details about shape.

## Slope adjustment

Consider a dataset of values {log $A_e^i$, log( $\sqrt{T}^i$ $A_t^i$)}, with i = 1..N, for a specific partition P. To allow for comparison with other partitions, we introduced the correction to $A_e$'and $A_t$':

$$A_e'^P = \frac{4\pi}{I_G^P} A_e^P \text{ and } A_t'^P = \frac{4\pi}{I_G^P} A_t^P$$

The correction factor, $4\pi/I^P_K$, is not the same for all data points (e.g. due to estimation errors), and will follow some distribution. There will be an uncorrelated Gaussian component to this distribution that will introduce a systematic error in the slope estimations, and a correlated

component that may genuinely alter the slope. Since in the $\{log\ A_e, log\ \sqrt{T}A_t\}$ plane this correction happens along the direction $\{\frac{1}{\sqrt{2}}, \frac{1}{\sqrt{2}}\}$, the variance introduced by its uncorrelated Gaussian component will also be only along the same direction, adding to the covariance matrix of the dataset a term we can later explicitly remove:

$$\sigma_c^2 = \sigma_{log\ I_G^P}^2\{\frac{1}{\sqrt{2}}, \frac{1}{\sqrt{2}}\} \otimes \{\frac{1}{\sqrt{2}}, \frac{1}{\sqrt{2}}\} = \frac{\sigma_{log\ I_G^P}^2}{2}\begin{pmatrix} 1 & 1 \\ 1 & 1 \end{pmatrix}$$

So, if $\sigma'^2_P$ is the covariance matrix for our dataset in the partition after applying the correction factor,

$$\sigma'^2_P = \begin{pmatrix} \langle(\log A_e)^2\rangle - \langle\log A_e\rangle^2 & \langle\log A_e \log\sqrt{T}A_t\rangle - \langle\log A_e\rangle\langle\log\sqrt{T}A_t\rangle \\ \langle\log A_e \log\sqrt{T}A_t\rangle - \langle\log A_e\rangle\langle\log\sqrt{T}A_t\rangle & \langle(\log\sqrt{T}A_t)^2\rangle - \langle\log\sqrt{T}A_t\rangle^2 \end{pmatrix}$$

Then the adjusted covariance matrix, with the systematic error removed, will be simply $\sigma''^2_P = \sigma'^2_P - \sigma_c^2$. The best linear fit, the one that minimizes the sum of squared residuals, will naturally lie perpendicular do the direction of minimal variance of the dataset after the adjustment, and therefore along the direction of the principal eigenvector of $\sigma''^2_P$. The slope $\alpha$ of this eigenvector will thus be the slope we seek. This can be obtained analytically for a self-adjoint positive 2×2 matrix such as this, expressed in terms of the components of $\sigma'^2_P$ and $\sigma_{log\ I_K^P}^2$, resulting in:

$$\alpha_{\text{Lobes}} = \frac{1}{\gamma + \sqrt{1 + \gamma^2}}$$

Where

$$\gamma = \frac{\sigma_{11}^2 - \sigma_{22}^2}{2\sigma_{12}^2 - \sigma_{\log I_G^P}^2}$$

Note that this adjustment introduces minimal changes to the data. Below we show the slope estimates for individual hemispheres (HCP data, age 26-30) with and without this correction scattered against each other. As expected, the magnitude of the adjustment is also correlated with the value of the slope, as a variance term along the regression line will not affect the slope.

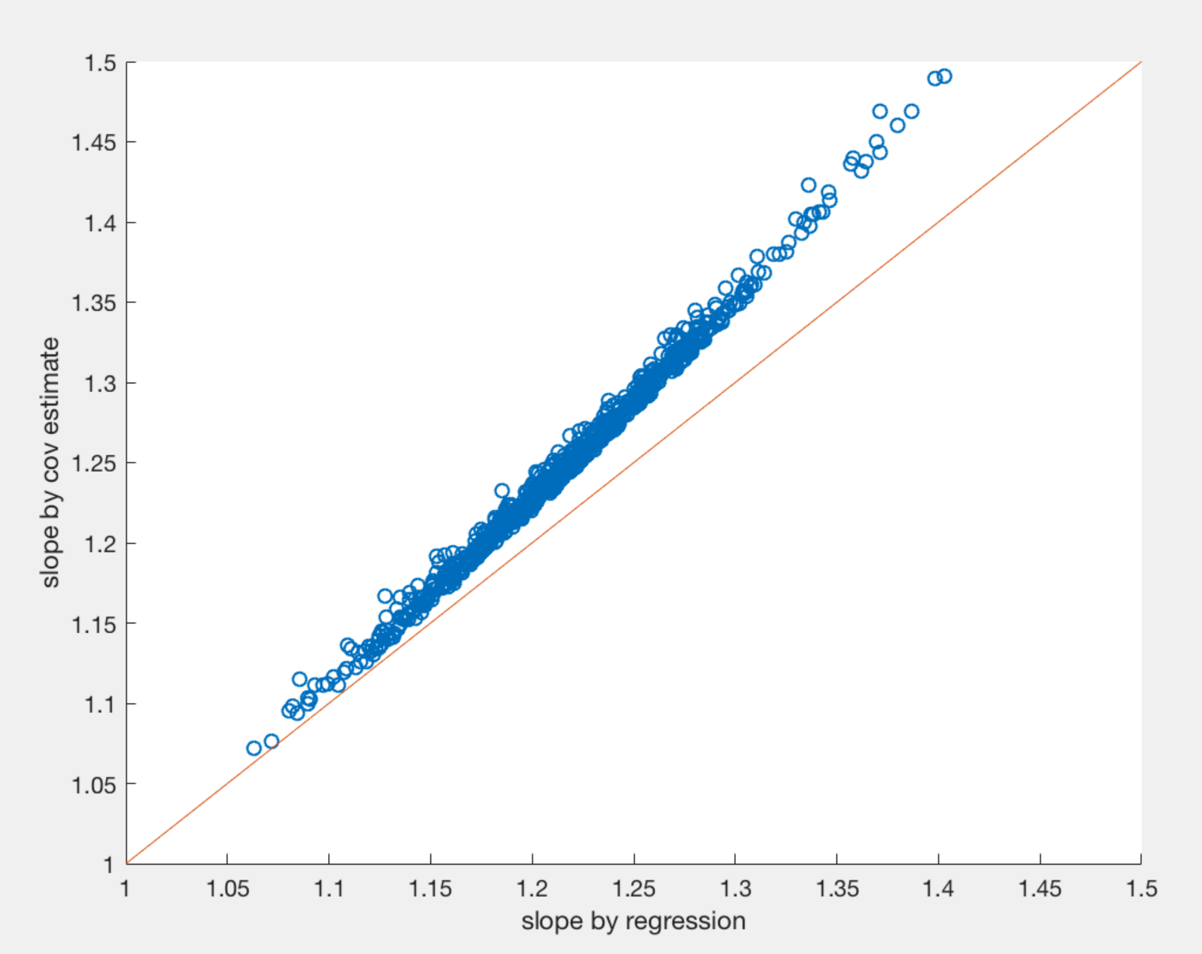


## Suppl. Text F

### *Data sources*

We used four publicly available datasets in this study. The **HCP** dataset comprises the 900 subject release from the Human Connectome Project (www.humanconnectome.org). Data were provided in part by the Human Connectome Project, WU-Minn Consortium (Principal Investigators: David Van Essen and Kamil Ugurbil; 1U54MH091657) funded by the 16 NIH Institutes and Centers that support the NIH Blueprint for Neuroscience Research; and by the McDonnell Center for Systems Neuroscience at Washington University.

The **NKI** data [Nooner *et al.* 2012] has been obtained from the Nathan Kline Institute (NKI) Rockland Sample (http://fcon_1000.projects.nitrc.org/indi/pro/nki.html), where funding for key personnel was provided in part by the New York State Office of Mental Health and Research Foundation for Mental Hygiene. Additional project support was provided by the NKI Center for Advanced Brain Imaging (CABI), the Brain Research Foundation (Chicago, IL), the Stavros Niarchos Foundation, and NIH grant P50 MH086385-S1.

The **ADNI** data has been obtained from the Alzheimer's Disease Neuroimaging Initiative (http://adni.loni.usc.edu/). Data collection and sharing for the ADNI project was supported by ADNI (National Institutes of Health Grant U01 AG024904). We included subjects from ADNI1, ADNI GO, and ADNI2 [Jack *et al.* 2010], and selected all 3T sessions. For all subjects

we only included one scan point (first 3T scan), to be consistent with the previous three cross-sectional datasets. We also only included the healthy controls and the Alzheimer's patients in this study.

The **IXI** data has been obtained from the brain development team at Imperial College London. This data was made available under the Creative Commons CC BY-SA 3.0 license and can be found at: http://brain-development.org/ixi-dataset/. Only healthy subjects scanned at Guy's hospital were included in this study, as this subset contains the most number of subjects.

As we only used publicly available datasets, no informed consent procedure was required. We confirm that we complied with all the data usage policies of each of the datasets we used. A general ethical approval was granted by Newcastle University to carry out the described research under the reference number 1186/2015. Details (e.g. field strength, voxel size etc.) for all the datasets can be found in Table 1.

### *Data processing*

For all datasets we used Freesurfer (http://surfer.nmr.mgh.harvard.edu/) for processing. We ran the Freesurfer recon-all pipeline on all subjects in the NKI, ADNI and IXI datasets. For the HCP dataset, we used the preprocessed package provided by the human connectome project, which already includes the Freesurfer results. Details regarding the preprocessing can be found in [Glasser et al. 2013].

To find the exposed surface of the full hemispheres, we ran the local gyrification pipeline in Freesurfer with the standard settings, and use the surfaces *h.pial-outer-smoothed produced by that pipeline. For a small number of subjects this pipeline failed and these subjects were simply excluded from our analysis.

### *Cortical thickness measurement*

We loaded the grey matter surface produced by Freesurfer (*h.pial) and the cortical thickness (*h.thickness) into Matlab, and matched each vertex in the surface mesh to their corresponding thickness. We then determined triangles in the surface mesh with zero thickness (i.e., with at least one vertex with zero thickness) and excluded them from subsequent analyses. As a last step we calculated the average vertex thickness for each remaining triangle, and the total average cortical thickness as a weighted average of all the triangle thicknesses. Note that the weight for each triangle is the proportion of its size relative to all other triangles. We also average the weight for the pial and the white matter surface triangles. The conversion from vertex based thickness to triangle based thickness is to enable regionwise comparisons to the surface area or any ROI for present and future analyses.

### *Total and exposed surface area measurement*

The total exposed surface area was calculated by loading the *h.pial surface into Matlab. Again, we removed triangles with zero thickness (corpus callosum) and took the sum of the

remaining triangle areas. This is in agreement with the approach taken by previous comparative neuroanatomical studies [Mota *et al.* 2015].

The total exposed surface area was calculated by loading the *h.pial-outer-smoothed into Matlab. We find and remove the triangles on the exposed surface corresponding to the previously-removed zero-thickness triangles on the pial surface, and compute the sum of the remaining triangle surface areas. We use a heuristic to find the corresponding triangles on the outer smoothed surface, which is the same as we use to find the outer smoothed surface corresponding to a lobe (see next section). Visual inspection of the results shows a very good agreement in general. Additionally, Fig. 1 in our previous paper [Wang *et al.* 2016] shows that our data agrees well with the previous comparative neuroanatomy data obtained by manual labelling. For each subject, we thus obtain a datapoint for each hemisphere, which, as in the previous studies, we treat as individual datapoints. As each subject has exactly two datapoints, this should not distort the results.

### *Finding outer smoothed surface area for a lobe*

For our analysis, we parcellated the brain (pial surface) into four different lobes using the Freesurfer labels. To find a corresponding parcellation of the outer smoothed area we used the following algorithm: We loop through all smoothed surface vertices, and find the nearest pial surface vertex. We then assign same label of that pial surface vertex to the smoothed surface vertex. As the smooth surface is a very dense mesh, this method creates a very accurate parcellation on the smooth surface.

*Supplementary Table F.1: Details of the public datasets we used. For all the references, the links are provided.*

| **Dataset** | HCP | NKI | IXI (Guy's Hospital subset) | ADNI control | ADNI AD |
|---|---|---|---|---|---|
| **Data sample origin** | https://db.humanconnectome.org/app/template/Index.vm | http://fcon_1000.projects.nitrc.org/indi/pro/nki.html | http://brain-development.org/ixi-dataset/ | http://adni.loni.usc.edu/ | |
| **Primary publication** | Glasser *et al.* 2013 http://www.sciencedirect.com/science/article/pii/S1053811913005053 | Nooner *et al.* 2012 http://www.ncbi.nlm.nih.gov/pmc/articles/PMC3472598/ | N/A | Jack *et al.* 2010 http://www.ncbi.nlm.nih.gov/pmc/articles/PMC2886577/ | |
| **Number of subjects** | 526 | 207 | 314 | 235 | 199 |
| **Female** | 315 | 87 | 175 | 124 | 93 |
| **Male** | 211 | 120 | 139 | 111 | 106 |
| **Age range** | 22-36 (mean: 29.21) | 4-85 (mean: 35.01) | 20-86 (mean: 51) | 56-95 (mean: 74.60) | 56-91 (mean: 74.91) |
| **Voxel size** | 0.7 mm isotropic | 1 mm isotropic | 0.94 x 0.94 x 1.2mm | varied | |
| **Field strength** | 3 Tesla | 3 Tesla | 1.5 Tesla | 3 Tesla | 3 Tesla |
| **Scanning protocol** | MP-RAGE | MP-RAGE (http://fcon_1000.projects.nitrc.org/indi/pro/nki/NKI_MPRAGE_PROTOCOL.pdf) | http://brain-development.org/scanner-philips-medical-systems-gyroscan-intera-1-5t/ | MP-RAGE (http://adni.loni.usc.edu/methods/documents/mri-protocols/) | |
| **Scanner type** | Siemens (Skyra modified) | Siemens (Magnetom) | Phillips Medical Systems Gyroscan Intera | Differed across sites | |
| **Pre-processed data provided** | Freesurfer subjects created from T1 and T2 images | As Lim *et al.* 2013 http://cercor.oxfordjournals.org/content/25/6/1477 | Freesurfer subjects created from T1 and T2 images | Preprocessed (see http://adni.loni.usc.edu/methods/mri-analysis/mri-pre-processing/) | |
| **Freesurfer version** | 5.3 modified version | 5.0 | 5.3 | 5.3 | |

The dataset will also be available on Zenodo under the link [to be generated upon publication], or upon email request (yujiang.wang@ncl.ac.uk).

## Suppl. Text G

In the main manuscript, Fig. 1C we show a distribution of slopes derived for each individual hemisphere. Of course, as each slope is derived based on four data points (four lobes), the confidence interval on each individual slope is large, and it is difficult to tell if the slopes are significantly different from each other.

To address this shortcoming, we apply linear mixed effect modelling to estimate the confidence intervals of the group slope, and also test if individual slopes are significantly different to each other. Note all results reported below are for the same subjects as shown in Fig. 1C, i.e. HCP age 22-25 subjects. Similar results hold for other age ranges and for other datasets.

Note that for this analysis, we could not correct for the noisy estimation in the g direction (Suppl Text E, Section "Slope adjustment"), which was based on covariance of the group. Hence the mean slope estimates are slightly lower than 1.25, but the confidence intervals shown in the following give an estimate of the group slope confidence regardless.

We tested the following model:
lme: y ~ 1 + x + (1+x|hemispheres)
where y=log10(At * sqrt(T)), and x = log10(Ae).

The slope estimate is: 1.2167, with a lower bound of 1.2090 and an upper bound of 1.2244, representing 95% confidence intervals. This means that we expect the confidence intervals to fall around +/- 0.01 of the mean slope.

To further test if individual hemispheres have significantly different slopes to each other we tested the alternative random intercept model:
lme_alt: y ~ 1 + x + (1|hemispheres)

When comparing lme_alt vs lme using the maximum likelihood method, no significant difference could be found (p=0.51949), indicating that the mixed intercept model is as good as the mixed slope model. We interpret this as the individual slopes not differing significantly in estimating a group slope.
